# Supplementary material for: Edge Dynamics in Iron-Cluster Catalyzed Growth of Single-Walled Carbon Nanotubes Revealed by Molecular Dynamics Simulations based on a Neural Network Potential
Source: arXiv:2302.09264 ancillary file (2024-12-03)
Supplement: Supplementary file 1 [file figure-SI.pdf]

Supporting Information for

Catalyzed Growth of Single-Walled Carbon Nanotube

by Machine Learning Molecular Dynamics Simulation

Ikuma Kohata<sup>\*,1</sup>, Ryo Yoshikawa<sup>1</sup>, Kaoru Hisama<sup>2</sup>, and Shigeo Maruyama<sup>\*,1</sup>

<sup>1</sup>Department of Mechanical Engineering, School of Engineering, the University of Tokyo,

7-3-1 Hongo, Bunkyo-ku, Tokyo, Japan

<sup>2</sup>Research Initiative for Supra-Materials, Shinshu University, 4-17-1 Wakasato, Nagano,

Nagano 380-8553, Japan

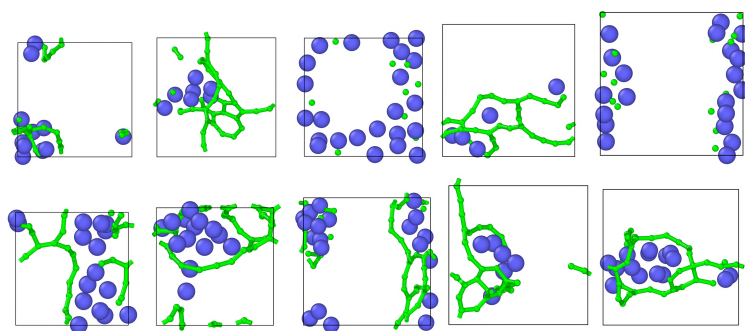

(a) Disordered structures.

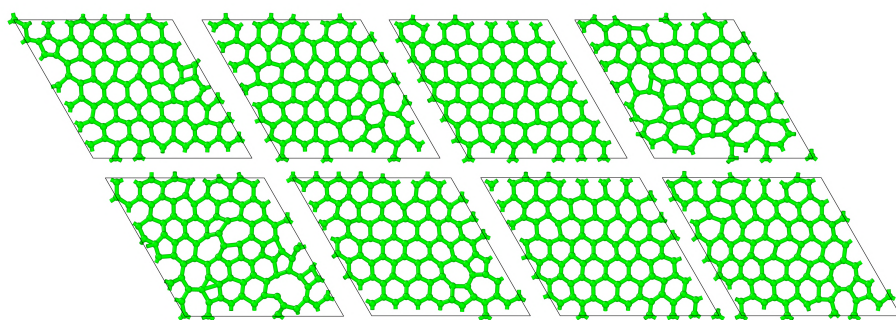

(b) Defective graphene structures.

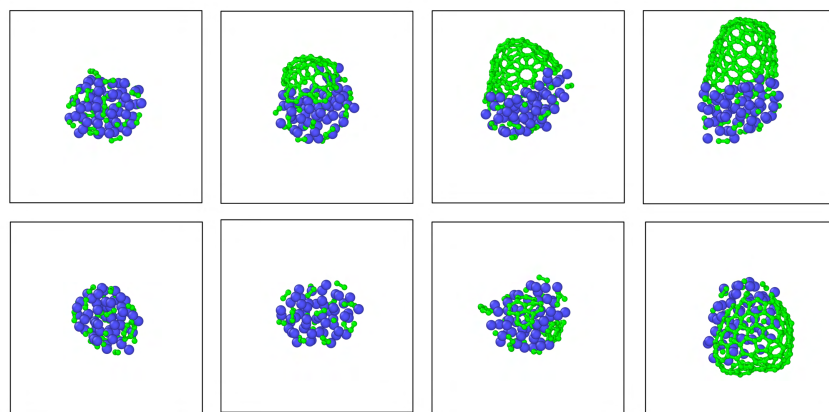

(c) CNT growth structures.

Figure S1: Examples structures sampled from the training dataset. The green and blue atoms represent carbon and iron, respectively.

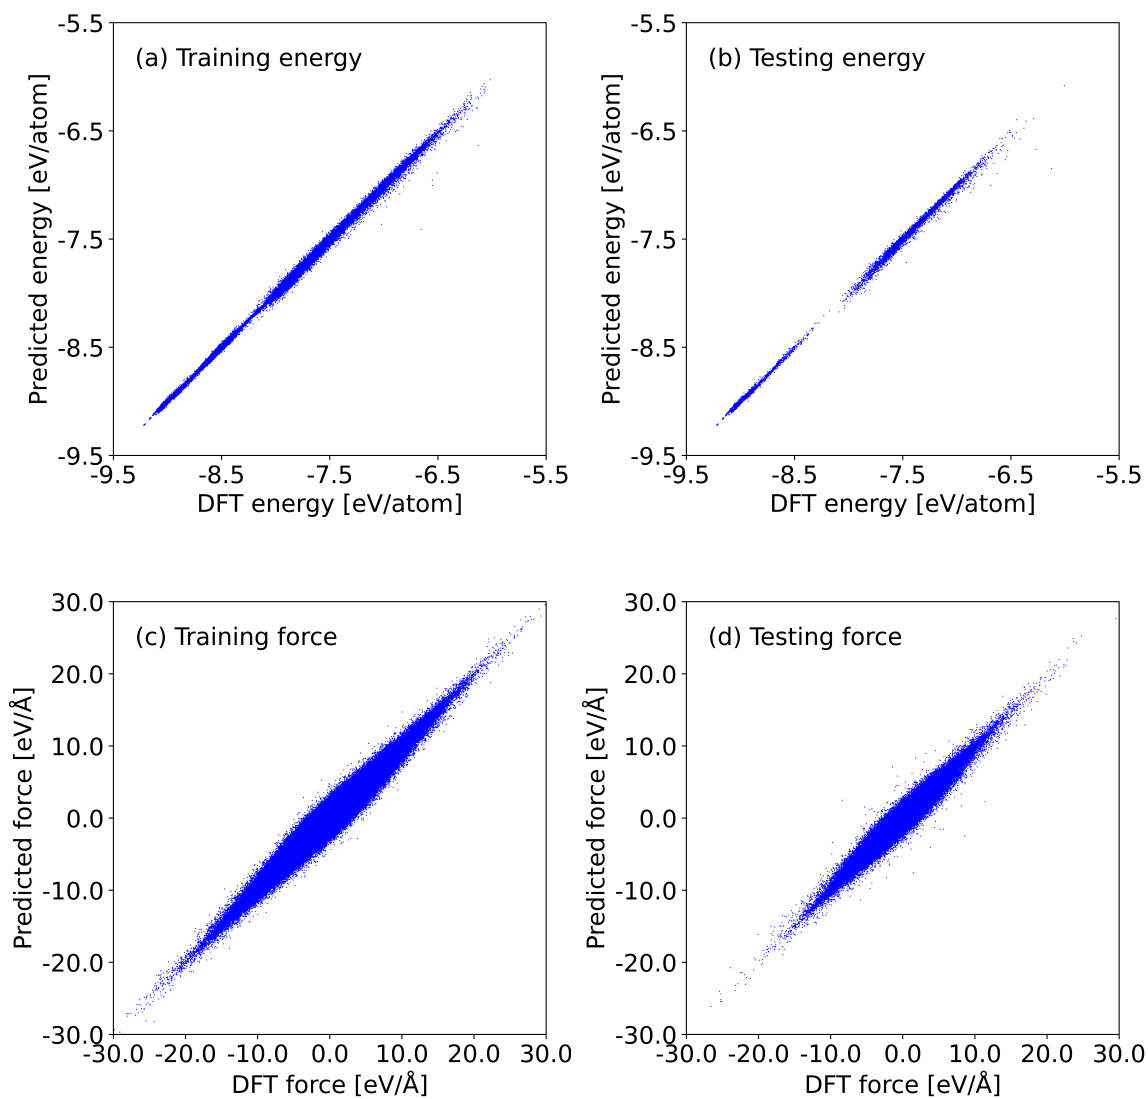

Figure S2: Comparison of total energies between DFT and NNP for (a) training and (b) testing dataset, and force comparison for (c) training and (d) testing datasets.

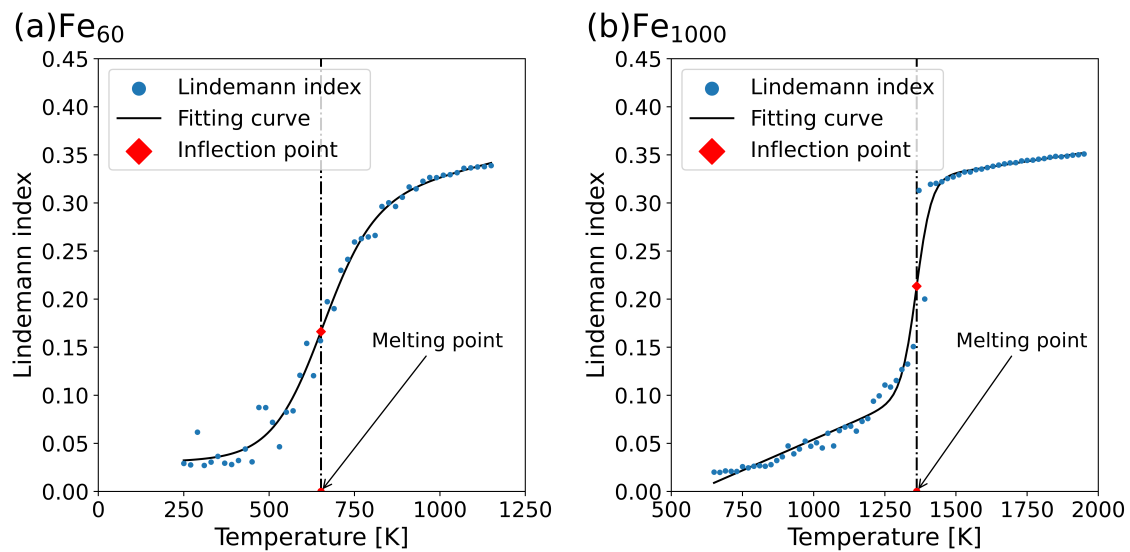

Figure S3: Lindemann index as a function of temperature for (a)  $\text{Fe}_{60}$  and (b)  $\text{Fe}_{1000}$  nanoparticles.

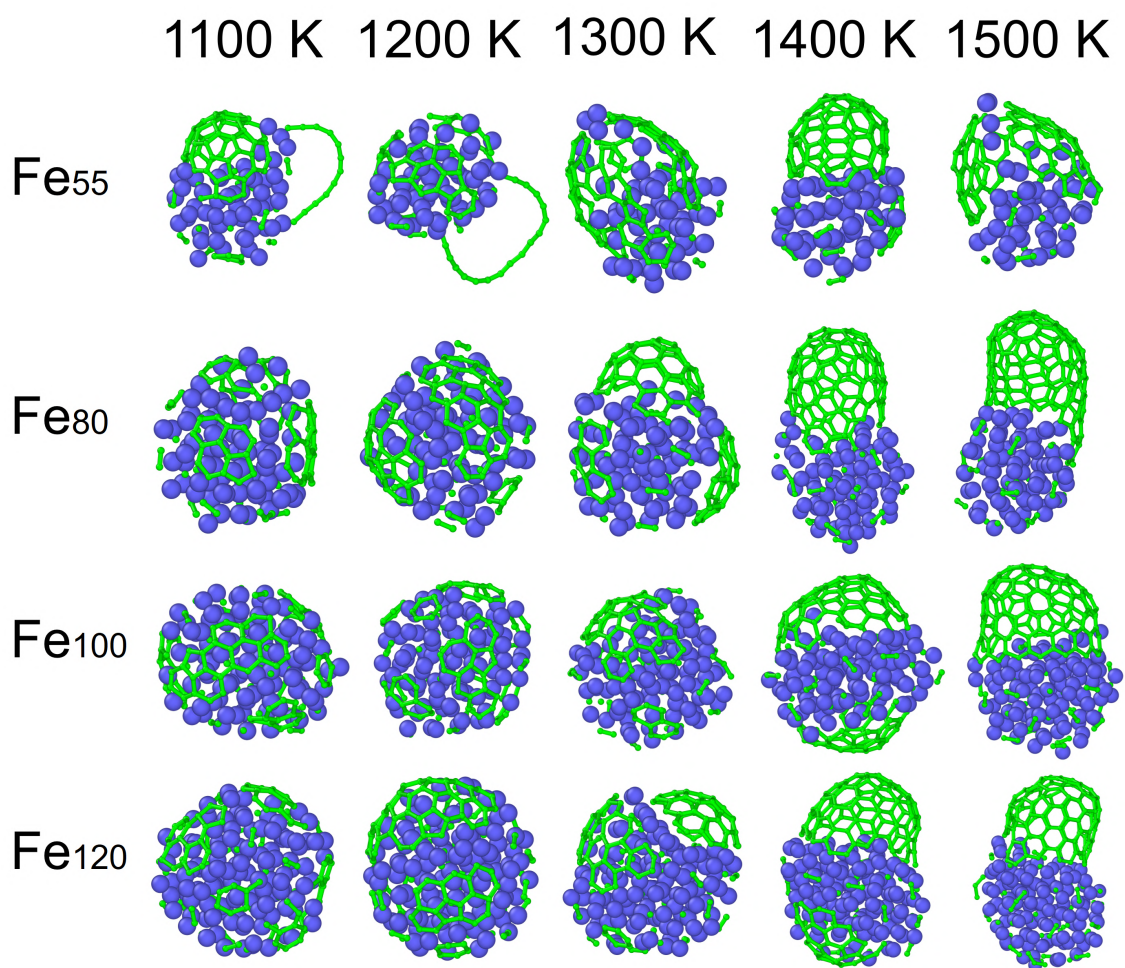

Figure S4: SWCNT growth trend by temperature and catalyst size. Each snapshot was taken after 80 ps of carbon supply.

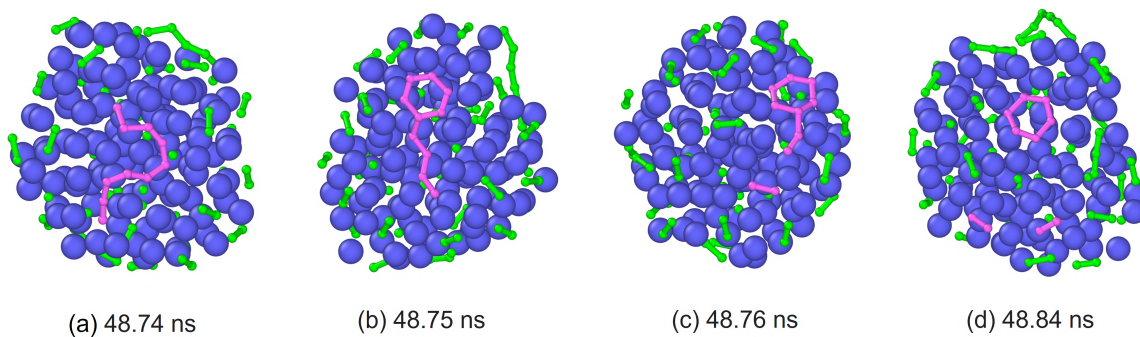

Figure S5: Snapshots of the first hexagon formation processes where the precursor is a 10-mer chain. The pink balls and polls represent carbon atoms and bonds composing the precursor chains, respectively.

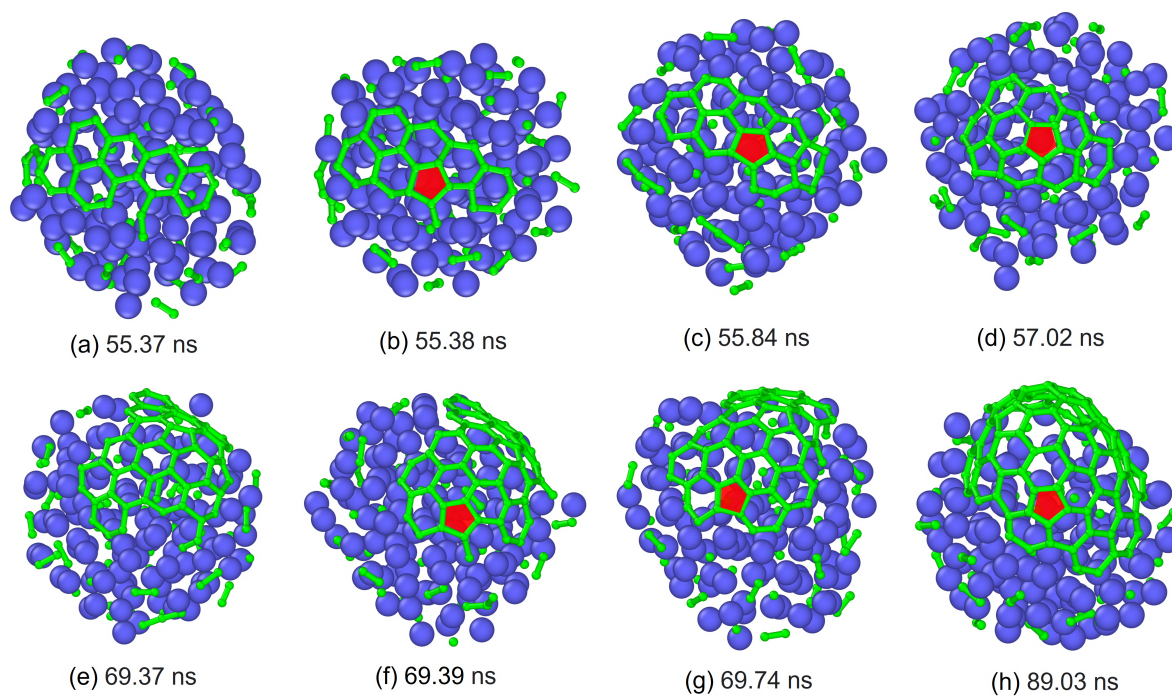

Figure S6: Snapshots of the pentagon formation processes. (a-d) The first pentagon formation. (e-f) The second pentagon formation.

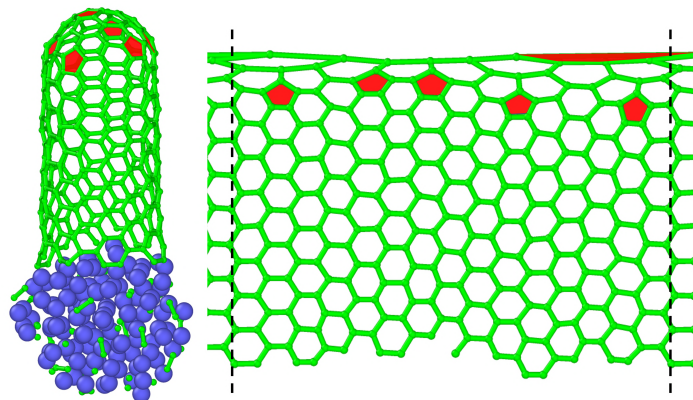

(a) (8,7) SWCNT grown at 1500 K from  $\text{Fe}_{120}$

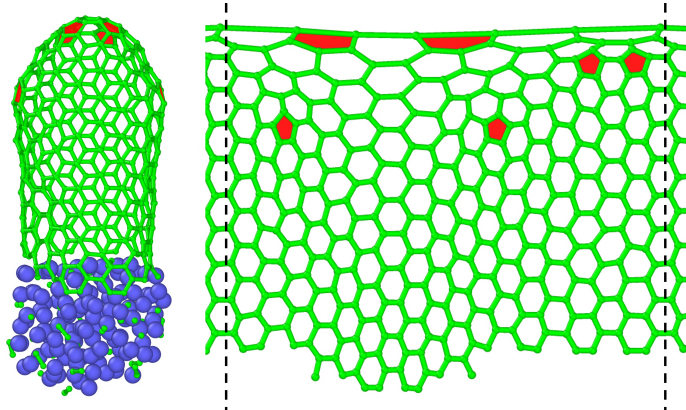

(b) (9,9) SWCNT grown at 1600 K from  $\text{Fe}_{120}$

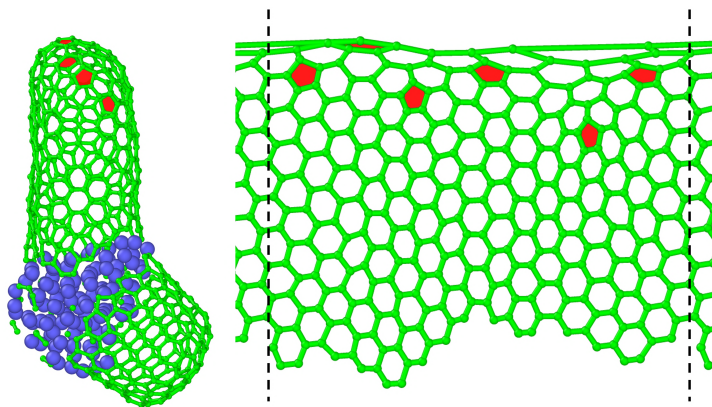

(c) (10,7) SWCNT grown at 1500 K from  $\text{Fe}_{120}$

Figure S7: Snapshots and developed views of defect-free SWCNTs. In the developed view, only C atoms included in the graphitic network were visualized, and C atoms included in the sub-cap beside (10,7) SWCNT were omitted for clarity.

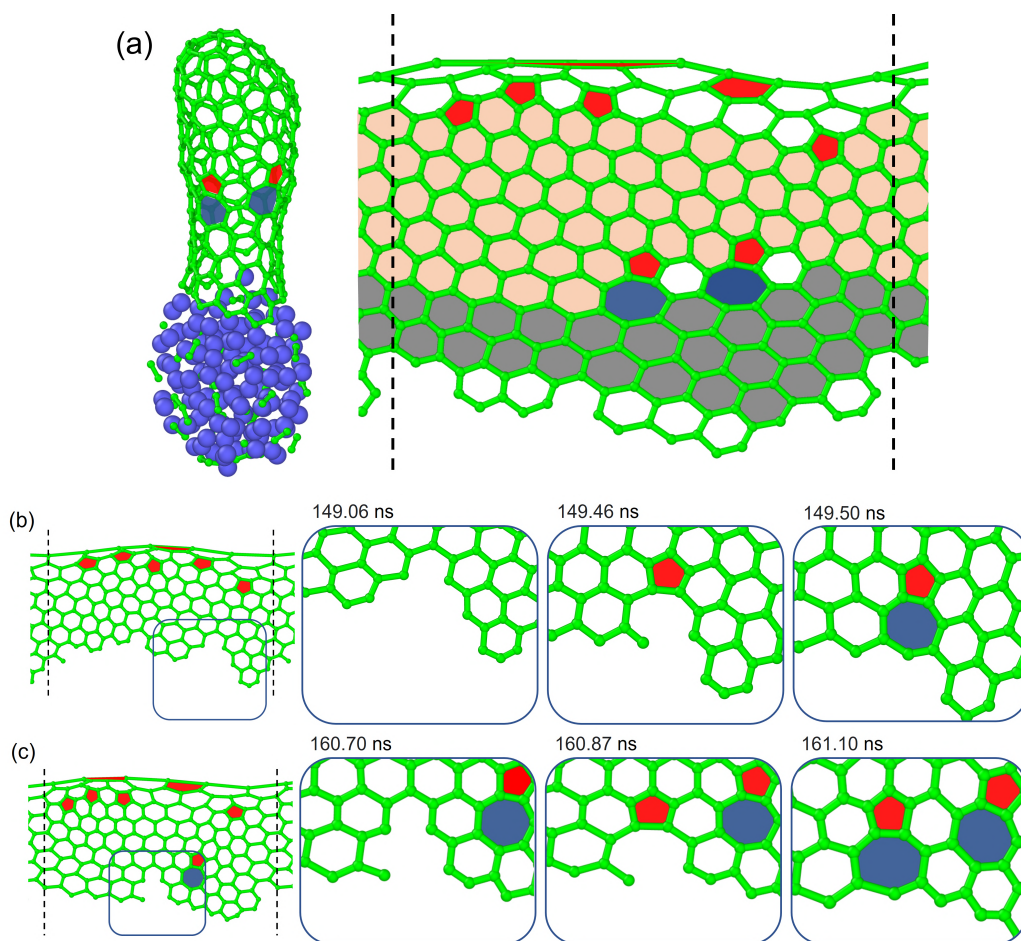

Figure S8: Snapshots of an SWCNT with 5-7 defect mediated chirality change. (a) Snapshot and developed view with chirality change from (10,3) to (8,3). (b) 5-7 defect formation process. The pale orange and gray areas are (10,3) and (8,3) sidewalls, respectively. The chirality of the white areas can not be assigned.
